# Supplementary material for: Tracing Equilibrium in Dynamic Markets via Distributed Adaptation
Source: arXiv:1804.08017 source file (2018-04-21)
Supplement: Supplementary file 1 [file appendix-misspending.tex]

\section{Misspending Potential Function}

Cole, Fleischer and Rastogi~\cite[Section 3.2]{CFR2010} proved that tatonnement updates lead to
linear convergence of the misspending potential function.
In this appendix, we give some intuition on how misspending potential function works.

First of all, recall the definition of gross-substitute (GS) Fisher market:
if one price $p_k$ increases, then the demand for every other good increases.
In other words, if one price $p_k$ increases, then the amount of money spent on every other good increases.
Since the total amount of money in the market is fixed, the amount of money spent on good $k$ decreases.

For static market, we normalize the supply of each good to be one unit.
Recall that $x_j$ denote the demand for good $j$, and $z_j := x_j - 1$ is the excess demand for good $j$.
The misspending function is $\phi(p) ~:=~ \sum_j p_j |z_j|$.
Let $s_j := p_j x_j$ denote the amount of money spent on good $j$.

\smallskip

\parabold{Intuition.}
We focus on the price update of one good, say good $1$.
We assume that $z_1$ is positive; the argument for the case of negative $z_1$ is symmetric.

When $z_1$ is positive, by tatonnement, we increase $p_1$ to some $p_1'$.
The new excess demand is $z_1'$, which is less than $z_1$.
For exposition purpose, we assume\footnote{This assumption is satisfied when the excess demand function is continuous.}
that the increment on the price is small enough such that $z_1'$ remains positive.
Then
$$
p_1 |z_1| - p_1' |z_1'| ~=~ p_1 \cdot (x_1 - 1) - p_1' \cdot (x_1' - 1) ~=~ s_1 - p_1 - s_1' + p_1' ~=~ (s_1 - s_1') + (p_1' - p_1).
$$
By the definition of GS, $(s_1 - s_1')$ is non-negative. Also, note that $p_1' - p_1$ is positive.
In other words, the first component of the misspending function decreases.

The other components of the misspending function might increase, though. However, note that
$$
\sum_{j\neq 1} \left(p_j |z_j| - p_j |z_j'|\right) ~\geq~ \sum_{j\neq 1} (s_j - s_j').
$$
and the RHS is exactly $-(s_1 - s_1')$, since the amount of money spent on all goods is fixed.

Thus, overall,
$$
\phi(p) - \phi(p') ~\geq~ (s_1 - s_1') + (p_1' - p_1) - (s_1 - s_1') ~\geq~ (p_1' - p_1),
$$
i.e., the misspending function decreases.

To domonstrate convergence upon synchronous price updates of all goods,
first we need that a tatonnement price update rule such that $p_j' - p_j = \Omega(p_j |z_j|)$;
rule \eqref{eq:multi-tat-update} suffices when the demand is not too high.
Second, as was done in~\cite[Section 3.2]{CFR2010}, is to carefully analyze the effect of one price update
on the other goods, so as to show that the synchronous updates yield an overall progress
which is proportional to the sum of progresses as made by hypothetically updating the price of only one good, for every good.

%We have just showed that the potential function value is non-increasing, but this is insufficient to guarantee convergence.
%To demonstrate convergence, one needs a stronger guarantee, say in the form of $\phi(p) - \phi(p') ~\geq~ \epsilon \cdot \phi(p)$.
%This can be achieved by assuming that the excess demand function is sufficiently smooth
%(by assuming that it has some ``elasticity'' parameters) and the tatonnement update rule is aggressive but not too aggressive.
